# Supplementary material for: Molecular Diffusion Replaces Capillary Pumping in Phase-Change Driven Nanopumps
Source: arXiv:1804.06056 ancillary file (2018-04-17)
Supplement: Supplementary file 1 [file Supplementary_information.pdf]

Supplementary Information for

# Molecular Diffusion Replaces Capillary Pumping in Phase-Change Driven Nanopumps

Yigit Akkus[a,b], Ali Beskok[a]

[a]Lyle School of Eng., Southern Methodist University, Dallas, Texas 75205, USA
[b]ASELSAN A.Ş., 06172 Yenimahalle, Ankara, Turkey

1. Methods
2. Pumping performance prediction in continuum scale
3. Density distribution of each system

# 1. Methods

Geometrically scaled, four different systems were simulated. The numbers of fluid (Ar) and solid (Pt) atoms in each system were; Pump-1: (990 Ar, 3280 Pt), Pump-2: (3990 Ar, 6480 Pt), Pump-3: (8663 Ar, 9680 Pt) and Pump-4: (14950 Ar, 12800 Pt). In each system, walls were composed of 4 solid layers and (1,0,0) crystal planes faced the liquid. The outermost layers of the walls were always fixed at their lattice positions. Periodic boundary conditions were applied in all directions. All simulations were carried out using Large-scale Atomic/Molecular Massively Parallel Simulator (LAMMPS) [1]. A time step of 5 fs was used and each collected data was averaged for 250 ps. Lennard-Jones (L-J) 6-12 potential was used to model the interactions between Ar-Ar and Ar-Pt atoms with molecular diameters of $\sigma_{Ar} = 0.34\,\text{nm}$, $\sigma_{Ar-Pt} = 0.3085\,\text{nm}$, and depth of the potential wells of $\varepsilon_{Ar} = 0.01042\,\text{eV}$, $\varepsilon_{Ar-Pt} = 0.00558\,\text{eV}$ [2]. L-J potential was truncated with a cut-off distance of $3\sigma_{Ar}$. Embedded atom model was utilized for Pt-Pt atomic interactions [3]. Simulations were started from the Maxwell-Boltzmann velocity distribution for all atoms at 110 K. In the first stage, Nosé-Hoover thermostat was applied to all atoms (except the outermost Pt layers) for 15 ns to stabilize the system temperature at 110 K. Then, microcanonical ensemble was applied to Ar atoms for 15 ns to equilibrate the system, while wall atoms were still subjected to the thermostat. At the end of this stage, stable liquid/vapor Ar mixture was obtained at 110 K. In order to determine the liquid-vapor interface, first, domain was divided to longitudinal slabs and average fluid density was calculated at each slab. Then, longitudinal slabs were divided into square bins and average fluid density was calculated for each bin. Starting from the outer gas phase regions, density of each bin was checked in positive and negative $x$-directions and the first bins, where the bin density exceeded the average slab density, were marked as the liquid-vapor interface. In the final stage, equal energy injection and extraction were applied to the solid atoms locating at the heating and cooling zones, respectively, for 40 ns. Other wall atoms were not allowed to vibrate in order to eliminate the heat conduction through solid wall. During heating/cooling, Ar atoms were subjected to microcanonical ensemble.

Molecular layering of fluid near a solid is actually an experimental observation [4]. Therefore, formation of this dynamic structuring during simulations should be considered as a link to the real-world behavior of the system. In all simulation stages, molecular layering of Ar is verified in the proximity of the walls. Moreover, the distribution and magnitude of density peaks were in a quite good agreement with the results of [2], where same L-J potential parameters were used.

## 2. Pumping performance prediction in continuum scale

The mass flow rate of a pressure induced laminar liquid flow in a channel of height, $h$, and width, $w$, is given by

$$\dot{m} = -\frac{h^3 w}{12\nu}\frac{dp}{dx} \ , \tag{S1}$$

where $\nu$ and $p$ are kinematic viscosity and pressure of the liquid, respectively. If the flow is driven by a capillary pressure gradient resulting from the asymmetric menisci at both ends of the channel, pressure gradient can be approximated using Young-Laplace equation:

$$\frac{dp}{dx} \simeq \frac{\sigma}{l}\Big(\frac{1}{R_{cond}} - \frac{1}{R_{evap}}\Big) \ , \tag{S2}$$

where $\sigma$ and $l$ are the surface tension coefficient and length of the channel, respectively. Radius of curvature, $R$, can be written as the functions of apparent contact angle, $\theta$ and channel height, $h$,

$$R = \frac{h/2}{\cos(\theta)} \ . \tag{S3}$$

Combination of Eqn. (S1), Eqn. (S2) and Eqn. (S3) yields the mass flow rate, $\dot{m}$, as the functions of apparent contact angles formed at the condenser and evaporator regions:

$$\dot{m} \simeq \frac{h^2 w}{6\nu}\frac{\sigma}{l}\Big[\cos(\theta_{evap}) - \cos(\theta_{cond})\Big] \ . \tag{S4}$$

Maximum theoretical mass flow rate, $\dot{m}_{max}^{therotical}$, which would be achieved if the heat conduction along the channel axis and heat loss from side walls are zero, requires that all of the heat input is utilized to evaporate the liquid from interface:

$$\dot{m}_{max}^{therotical} = \frac{\dot{q}_{evap}}{h_{fg}} \ . \tag{S5}$$

The ratio of actual mass flow rate to the theoretically maximum one is a good measure of the performance of the pump:

$$\eta \equiv \frac{\dot{m}}{\dot{m}_{max}^{therotical}} \ . \tag{S6}$$

When Eqn. (S4) and Eqn. (S5) are inserted to Eqn. (S6), performance of the pump can be demonstrated as the functions of both heat inputs and system geometry. After some algebraic manipulations, the pump performance can be shown as follows:

$$\eta \cong \Big(\frac{1}{12}\Big)\Big(\frac{\dot{q}_{evap}/2ew}{\sigma h_{fg}/\nu}\Big)^{-1}\Big(\frac{e}{h}\Big)^{-1}\Big(\frac{l}{h}\Big)^{-1}\Big[\cos(\theta_{evap}) - \cos(\theta_{cond})\Big] \ , \tag{S7}$$

where $e$ is the length of the heat addition region. Numerator of the second term at the right hand side is simply the applied heat flux to the liquid. Denominator of this term is a group of physical properties of the fluid. For a system with small temperature variations, this group can be considered as constant and utilized to non-dimensionalize the heat flux. Thus, the second term at the right hand side can be considered as non-dimensional heat flux, $\dot{q}''^{*}_{evap}$, applied to the system. The third and fourth terms, on the other hand, are scaled heat addition length, $e^*$, and aspect ratio of the channel, $l^*$, respectively. Therefore, Eqn. (S7) can be written in terms of these non-dimensional parameters as follows:

$$\eta \cong (\dot{q}''^{*}_{evap})^{-1} \left[ \frac{\cos(\theta_{cond}) - \cos(\theta_{evap})}{12 e^* l^*} \right] . \tag{S8}$$

Eqn. (S8) simply implies that if the applied heat flux and geometric similarity of the system are preserved, the pump should exhibit identical performance. However, this prediction is restricted with the continuum scale. When nanoscale effects are present, physical properties such as density [5] and viscosity [6] or geometrical parameters such as contact angle [7] exhibit considerable variations, which can affect the pump performance.

## 3. Density distribution of each system

Density distribution of Argon liquid/vapor mixture for each pump is given in Fig. S1. The liquid/vapor interfaces are conspicuous in each pump due to the density difference of the phases. Density gradient between evaporator and condenser regions are prominent within high density layers. For Pump-1, molecular layering is effective everywhere in the channel with five distinct high density layers and there exists no bulk liquid region. For the other pumps, liquid bulk region exists and the extent of molecular layering decreases with larger system sizes.

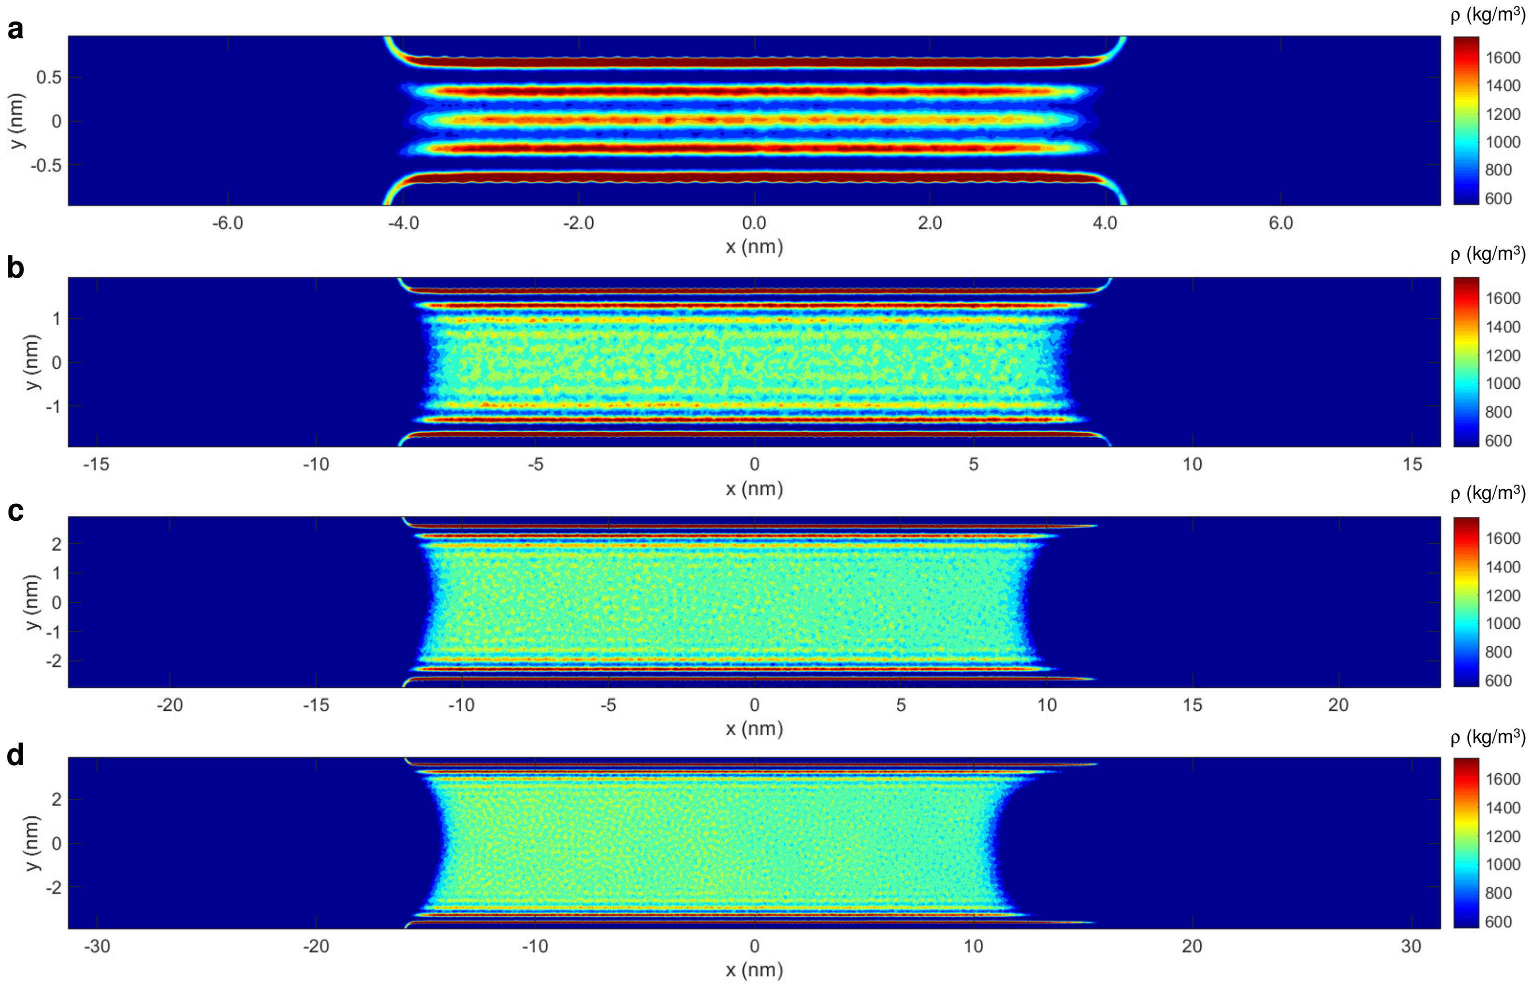


Figure 1: Ar density distribution between channel walls for (a) Pump-1, (b) Pump-2, (c) Pump-3 and (d) Pump-4. Wall regions are not included in the plots for brevity. In each plot, colour gradient is restricted for the data between $550\,\mathrm{kg/m^3}$ and $1750\,\mathrm{kg/m^3}$.

# References

[1] S. Plimpton. Fast parallel algorithms for short-range molecular dynamics. *J. Comput. Phys.*, 117(1):1–19, 1995.

[2] S. Maruyama and T. Kimura. A study on thermal resistance over a solid-liquid interface by the molecular dynamics method. *Therm. Sci. Eng.*, 7(1):63–68, 1999.

[3] S.M. Foiles, M.I. Baskes, and M.S. Daw. Embedded-atom-method functions for the fcc metals Cu, Ag, Au, Ni, Pd, Pt, and their alloys. *Phys. Rev. B*, 33(12):7983, 1986.

[4] F. Heslot, N. Fraysse, and A.M. Cazabat. Molecular layering in the spreading of wetting liquid drops. *Nature*, 338(6217):640, 1989.

[5] J. Ghorbanian, A.T. Celebi, and A. Beskok. A phenomenological continuum model for force-driven nano-channel liquid flows. *J. Chem. Phys.*, 145(18):184109, 2016.

[6] T.Q. Vo, M. Barisik, and B.H. Kim. Near-surface viscosity effects on capillary rise of water in nanotubes. *Phys. Rev. E*, 92(5):053009, 2015.

[7] M. Barisik and A. Beskok. Wetting characterisation of silicon (1, 0, 0) surface. *Mol. Simulat.*, 39(9):700–709, 2013.
